# Supplementary material for: Phase stability, chemical bonding and mechanical properties of titanium nitrides: A first-principles study
Source: arXiv:1411.1485 source file (2014-11-06)
Supplement: Supplementary file 1 [file Supplementary_materials.pdf]

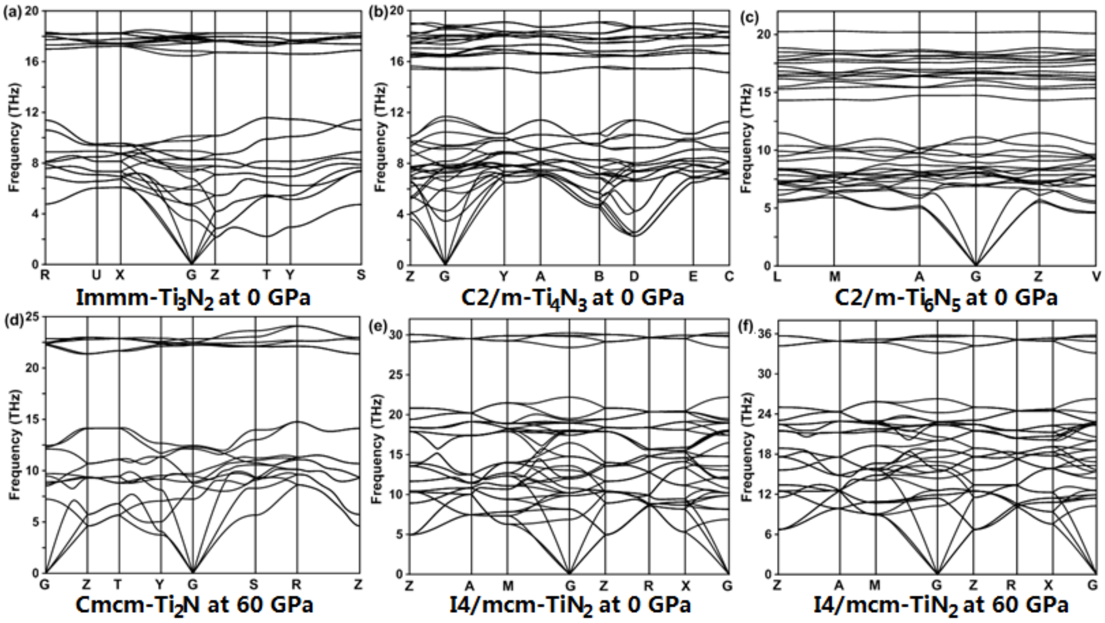


**Figure. 1s Calculated phonon dispersion curves for the Ti-N polymorphs**

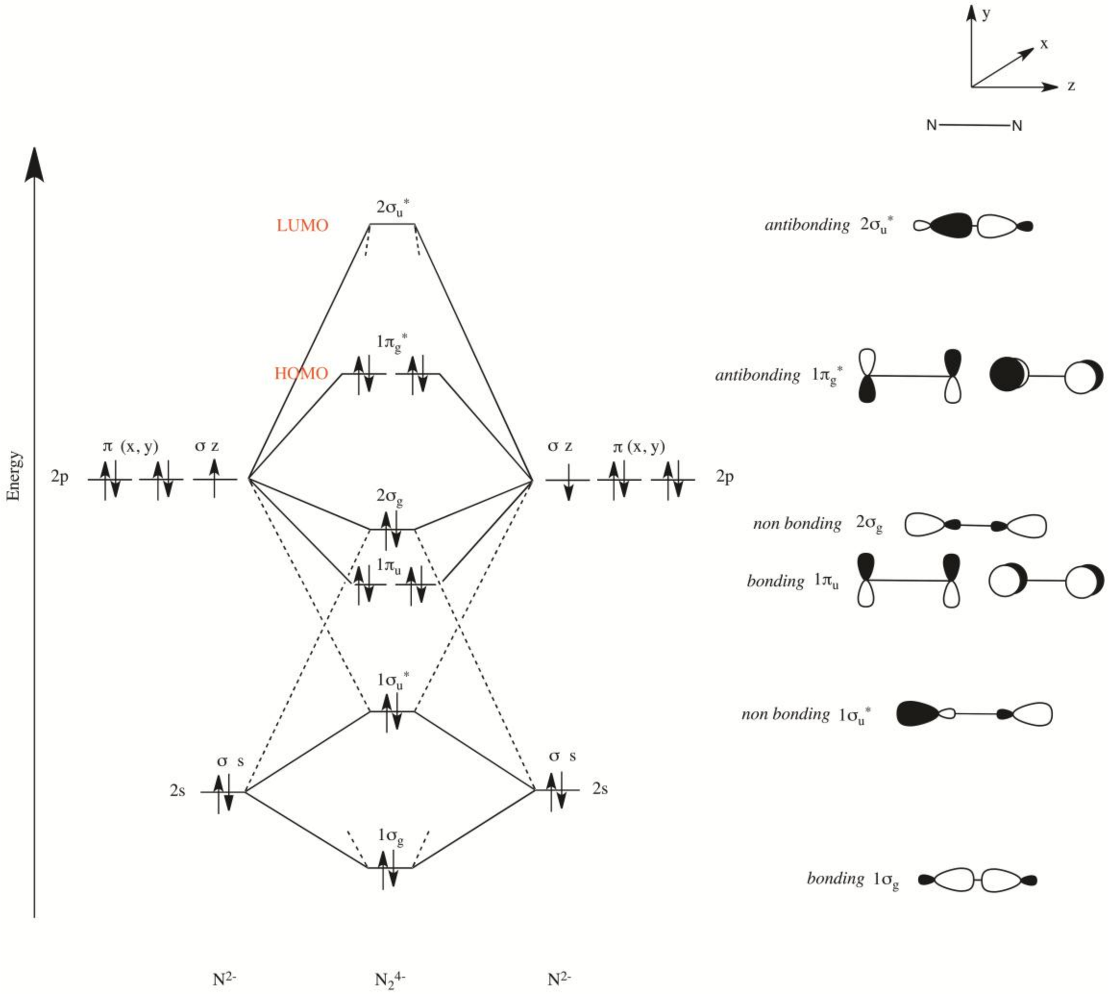


**Figure. 2s Schematic molecular orbital diagram of $N_2^{4-}$. The plain and dashed lines indicated the primary and secondary parentages of the orbitals, respectively (2s-2p$_z$**

**mixing). Only the valence orbitals are shown. $N_2^{4-}$ anion has 14 valence electrons (ve) and a bond order of 1.**

## Table. 1s Space group, lattice parameters, Wyckoff position, enthalpy of formation of Ti-N compounds

| Compounds | Pressure (GPa) | Lattice parameters | | | | Wyckoff position | | | | | ΔH |
|---|---|---|---|---|---|---|---|---|---|---|---|
| | | a | b | c | β | Atom | Site | x | y | z | (eV/atom) |
| $Ti_2N$ | 0 | 4.958 | | 3.037 | | Ti | 4g | 0.703 | 0.703 | 0.5 | -1.286 |
| *P4₂/mnm* → $P4_2/mnm$ | | 4.945[2] | | 3.034[2] | | N | 2b | 0 | 0 | 0.5 | |
| $Ti_3N_2$ | 0 | 4.156 | 3.035 | 9.160 | | Ti | 2d | 0.5 | 0 | 0.5 | -1.465 |
| *Immm* | | | | | | Ti | 4j | 0 | 0.5 | 0.316 | |
| | | | | | | N | 4i | 0 | 0 | 0.162 | |
| $Ti_4N_3$ | 0 | 9.934 | 3.018 | 10.302 | 150.3 | Ti | 4i | 0.266 | 0.5 | 0.633 | -1.549 |
| *C2/m* | | | | | | Ti | 4i | 0.258 | 0 | 0.885 | |
| | | | | | | N | 4i | 0.001 | 0.5 | 0.749 | |
| | | | | | | N | 2a | 0 | 1 | 1 | |
| $Ti_6N_5$ | 0 | 5.214 | 9.015 | 8.517 | 144.8 | Ti | 8j | 0.487 | 0.824 | 0.746 | -1.621 |
| *C2/m* | | | | | | Ti | 4i | 0.001 | 1 | 0.738 | |
| | | | | | | N | 4h | 1 | 0.335 | 0.5 | |
| | | | | | | N | 4g | 0.5 | 0.166 | 0 | |
| | | | | | | N | 2c | 1 | 0 | 0.5 | |
| TiN | 0 | 4.255 | | | | Ti | 4a | 0 | 0 | 0 | -1.671 |
| *Fm-3m* | | 4.246[1],4.25[3] | | | | N | 4b | 0 | 0.5 | 1 | |
| $Ti_2N$ | 60 | 2.78 | 10.545 | 4.027 | | Ti | 4c | 0.5 | 0.318 | 0.25 | -2.103 |
| *Cmcm* | | | | | | Ti | 4c | 1 | 0.452 | 0.75 | |
| | | | | | | N | 4c | 0.5 | 0.317 | 0.75 | |
| $TiN_2$ | 60 | 4.148 | 5.033 | | | Ti | 4a | 0.5 | 0.5 | 0.75 | -2.347 |
| *I4/mcm* | | | | | | N | 8h | 0.615 | 0.885 | 1 | |

## Equations: The directional dependence of the Young's modulus for crystals of different symmetries

$$\frac{1}{E_{Cubic}} = s_{11} - 2(s_{11} - s_{12} - \frac{1}{2}s_{44})(l_1^2 l_2^2 + l_2^2 l_3^2 + l_3^2 l_2^2)$$

$$\frac{1}{E_{Tetra}} = (l_1^4 + l_2^4)s_{11} + l_3^4 s_{33} + l_1^2 l_2^2 (2s_{12} + s_{66}) + l_3^2(1 - l_3^2)(2s_{13} + s_{44})$$

$$\frac{1}{E_{Orth}} = l_1^4 s_{11} + l_2^4 s_{22} + l_3^4 s_{33} + l_1^2 l_2^2 (2s_{12} + s_{66}) + l_2^2 l_3^2 (2s_{23} + s_{44}) + l_1^2 l_3^2 (2s_{13} + s_{55})$$

$$\frac{1}{E_{Orth}} = l_1^4 s_{11} + l_2^4 s_{22} + l_3^4 s_{33} + 2(l_1^2 l_2^2 s_{12} + l_2^2 l_3^2 s_{23} + l_1^2 l_3^2 s_{13}) + l_2^2 l_3^2 s_{44} + l_1^2 l_3^2 s_{55}$$
$$l_1^2 l_2^2 s_{66} + 2 l_1 l_2 (l_1^2 s_{16} + l_2^2 s_{26} + l_3^2 (s_{36} + s_{45}))$$

where $S_{ij}$ are the elastic compliance tensor components constants and $l_1$, $l_2$ and $l_3$ are the

direction cosines.

## Reference


1. Liu K, Zhou X L, Chen H H, et al. Structural and elastic properties of TiN under high pressure[J]. Physica B: Condensed Matter, 2012, 407(17): 3617-3621.
2. Holmberg B. Structural studies on the titanium-nitrogen system [J]. Acta Chemica Scandinavica, 1962, 16(5): 13.
3. Lazar P, Redinger J, Podloucky R. Density functional theory applied to VN/TiN multilayers [J]. Physical Review B, 2007, 76(17): 174112.
